# Supplementary material for: FEABench: Evaluating Language Models on Multiphysics Reasoning Ability
Source: arXiv:2504.06260 source file (2025-04-08)
Supplement: Supplementary file 1 [file ft.tex]

\section{Does fine-tuning boost performance?}
\label{app:ft}
\newcommand{\Nsmall}[1]{\leavevmode{\color{gray}#1}}

\begin{table}
\centering
\caption{Code Metrics: Before and after Fine-Tuning Gemini-1.5-Flash-001.}
\begin{tabular}{p{1.2in}p{.7in}p{.7in}p{.9in}p{1in}}
\toprule
Description & Executability & Model Tree Score & Code Similarity & Valid Target \\
\midrule
FT $|$ Zero-Shot & 0.50$\pm$0.06 & 0.24$\pm$0.06 & 0.10$\pm$0.02 & 0/15 \\
Baseline $|$ Zero-Shot & 0.08$\pm$0.03 & 0.16$\pm$0.05 & 0.08$\pm$0.01 & 0/15 \\
% FT $|$ One-Shot & \textbf{0.57}$\pm$0.07 & 0.14$\pm$0.04 & 0.11$\pm$0.01 & 0/15 \\
\midrule
Baseline $|$ One-Shot & \textbf{0.57}$\pm$0.04 & \textbf{0.49}$\pm$0.06 & \textbf{0.14}$\pm$0.02 & 0/15 \\
\bottomrule
\end{tabular}
\end{table}

\begin{table}
\centering
\caption{Physics Metrics: Before and after Fine-Tuning Gemini-1.5-Flash-001.}
\begin{tabular}{p{1.2in}p{.75in}p{.6in}p{.6in}p{.7in}p{.7in}}
\toprule
Description & Interface Factuality & Interface Recall & Feature Recall & Feature Property Recall & Feature Dimension \\
\midrule
FT $|$ Zero-Shot & 0.42$\pm$0.15 & 0.36$\pm$0.13 & 0.13$\pm$0.09 & \textbf{0.15}$\pm$0.09 & \Nsmall{-} \\
Baseline $|$ Zero-Shot & \Nsmall{-} & 0$\pm$0 & 0.20$\pm$0.11 & 0.07$\pm$0.07 & \Nsmall{-} \\
\midrule
% FT $|$ One-Shot & 0.29$\pm$0.18 & 0.14$\pm$0.10 & 0.10$\pm$0.07 & 0.00$\pm$0.00 & \Nsmall{1.00$\pm$nan} \\
Baseline $|$ One-Shot & \textbf{0.80}$\pm$0.11 & \textbf{0.71}$\pm$0.13 & \textbf{0.36}$\pm$0.11 & 0.01$\pm$0.01 & \textbf{0.53}$\pm$0.18 \\
\bottomrule
\end{tabular}
\end{table}

\cready{The unfamiliarity of LLMs with permissible options and arguments to the \comsol calls is a significant factor contributing to the difficulty of the benchmark. This raises the prospect of exploring whether fine-tuning can boost the performance of LLMs on generating code. We used the Google AI Studio platform \citep{gaistudio} to tune the `gemini-1.5-flash-001-tuning' checkpoint on 180 problems in \benchlarge{} for 5 epochs. This platform imposed a limit of $4\times10^4$ characters on the inputs and $5000$ characters on the outputs. All but two of the 180 \benchlarge{} code outputs exceed this limit. We used a shorter, Zero-Shot prompt (without the One-Shot example) and truncated the dataset's inputs and outputs to adhere the limit during fine-tuning.

At inference time, we examine three LLMs x Prompting scenarios in terms of their performance on the \benchmain{} problems and on the task \model, namely (1) Baseline $|$ Zero-Shot: the untuned checkpoint (`gemini-1.5-flash-001-tuning') paired with a Zero-Shot prompt similar to that used during training (2) FT $|$ Zero-Shot: the Fine-Tuned model paired with the same prompt and, (3) Baseline $|$ One-Shot: the untuned checkpoint paired with the One-Shot prompt used in other experiments in this paper.

With the Zero-Shot prompt, the untuned LLM performs abysmally on several metrics including Executability. This is unsurprising, since the LLM sees no template for how its code should be structured. In this setting, the Fine-Tuned LLM seems to offer advantages, in terms of enabling the LLM to generate more executable code (Executability: 0.08 $\rightarrow$ 0.50). However, the untuned LLM prompted with the One-Shot example outperforms the fine-tuned LLM across most metrics, especially evident in the stark difference in the Physics Recall Metrics and the Model Tree Score. 

The failure of fine-tuning in yielding significant gains can be attributed to several factors in this experiment. First, the fine-tuned checkpoint overfits to the training distribution. Even when the code is reasonably `executable' (0.50), it is likely misaligned with what the prompt actually requires the LLM to do -- observe the Model Tree Score is 0.24 (FT) vs 0.49 (Baseline $|$ One-Shot). This was also qualitatively noticeable since the outputs during inference were also truncated midway, similar to the truncated outputs in the training distribution. 

Using the same checkpoint's tokenizer, the median number of tokens in the input zero-shot prompt and the output code, (before truncation) is 4036 and 7122 tokens respectively, across the 180 problems. The limits imposed during fine-tuning exacerbate the performance of the fine-tuned LLM. Since the linewise mapping of the inputs (natural language modeling instructions) to code is not one-to-one, the truncation only allows the LLM to see the first chunk of the correct answer. Lastly, the training distribution is not identical to the test-time distribution: the \benchlarge{} inputs use API-specific explicit instructions from the tutorials. The problem descriptions corresponding to \model are concise problem descriptions.
}
